# Supplementary material for: Observation of spin-orbit coupling induced Weyl points and topologically protected Kondo effect in a two-electron double quantum dot
Source: arXiv:1804.06447 ancillary file (2018-04-17)
Supplement: Supplementary file 1 [file SupplementaryInformation-v8.pdf]

# Supplementary Information for:
# „Observation of spin-orbit coupling induced Weyl points and topologically protected Kondo effect in a two-electron double quantum dot"


Zoltán Scherübl,[1] András Pályi,[2,3] György Frank,[1] István Lukács,[4] Gergő Fülöp,[1] Bálint Fülöp,[1] Jesper Nygård,[5] Kenji Watanabe,[6] Takashi Taniguchi,[6] Gergely Zaránd,[3] and Szabolcs Csonka[1]

*[1]Department of Physics, Budapest University of Technology and Economics and MTA-BME "Momentum" Nanoelectronics Research Group, H-1111 Budapest, Budafoki út 8., Hungary*
*[2]Department of Physics, Budapest University of Technology and Economics, H-1111 Budapest, Hungary*
*[3]Exotic Quantum Phases "Momentum" Research Group, Budapest University of Technology and Economics, H-1111 Budapest, Hungary*
*[4]Center for Energy Research, Institute of Technical Physics and Material Science, Budapest, Hungary*
*[5]Center for Quantum Devices and Nano-Science Center, Niels Bohr Institute, University of Copenhagen, Universitetsparken 5, DK-2100 Copenhagen, Denmark*
*[6]National Institute for Material Science, 1-1 Namiki, Tsukuba, 305-0044, Japan*


## I. SAMPLE

Schematics of the device are shown in Fig. S1. Altogether 12 of the bottom gates were contacted, from which 3 were placed on each side of the device below the normal contacts, and have been used as a single gate. Gates $g_2$, $g_4$, and $g_6$ were used to define the confinement potential of the double dot in the nanowire, while $g_3$ and $g_5$ served as left and right plunger gates (noted with $g_L$ and $g_R$ in the main text). Large ($\sim 1$ V) positive values were applied on $g_1$, $g_7$ and $g_8$ to induce a highly transmitting wire segment between the normal electrodes and the QDs.

E-beam lithography of fine bottom gates was carried out by 600K PMMA resist with thickness of 50 nm using cold development process ($-10$°C). High quality wurtzite InAs nanowires with diameter of 80 nm grown by solid-source molecular beam epitaxy,[1] an optimized process to suppress stacking faults[2] were used. Before cool down, the sample holder was carefully pumped during night to remove adsorbed water layer from the wire surface to avoid random potential profile along the wire and to reduce charge fluctuations. In earlier bottom gated devices $SiN_x$ or $HfO_2$ were used as an insulating layer between the gate electrodes and the nanowire. Charge traps formed in the polycrystalline insulator introduced instabilities during the measurements. Here we choose exfoliated hexagonal boron-nitride (hBN) as an insulating layer, for which we expected to have higher stability due to the better crystalline structure. Indeed, the stability of the device was remarkable, we were able to characterize the same charge state through out several weeks.

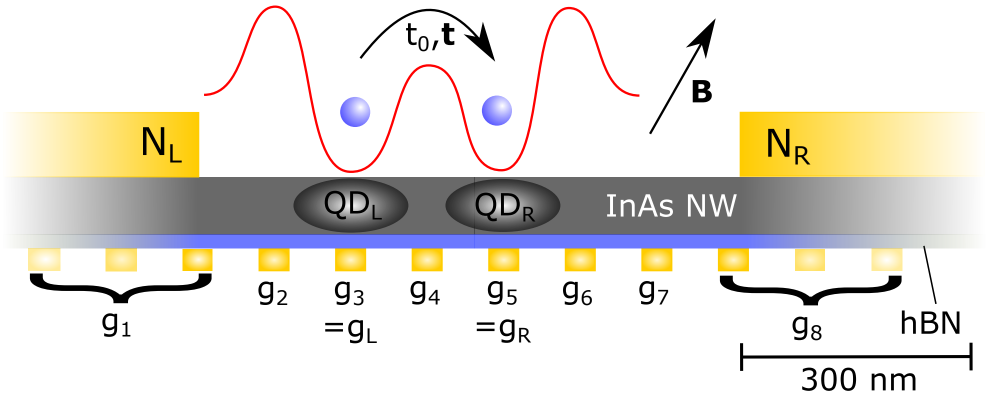


FIG. S1: a) Cross section of the device with proper dimension (see scale bar).

## II. ADDITIONAL DATA ON THE MAGNETIC FIELD DEPENDENCE OF THE GAP

In Fig. 2d and e of the main text, we presented inelastic co-tunneling spectroscopy data, which describes the magnetic field dependence of the energy gap between the ground and first excited states in the (1,1) charge state.

There, the measured differential conductance is shown as the function of the strength of the magnetic field $B$ and the bias voltage $V_{\mathrm{bias}}$. Here, we provide additional data of the same kind, taken at various orientations of the magnetic field. We have performed this measurement by varying the magnetic field polar angle $\theta$ in steps of $10°$ between $0°$ and $180°$, and tuning the azimuthal angle $\phi$ to 4 different values $\phi = -45°, 0°, 45°, 90°$. (See Fig. 2a for the definition of the reference frame.) An overview of the measured conductance maps is shown in Fig. S2 along the meridian of longitude $\phi = 90°$ (two top rows) and a circle at latitude $\theta = 70°$ (bottom row). Note that the conductance units are $G_0 = 2e^2/h$. Colors of the frames of the measurement panels refer to the magnetic field orientation, and corresponds to the balls indicated in the top right panel.

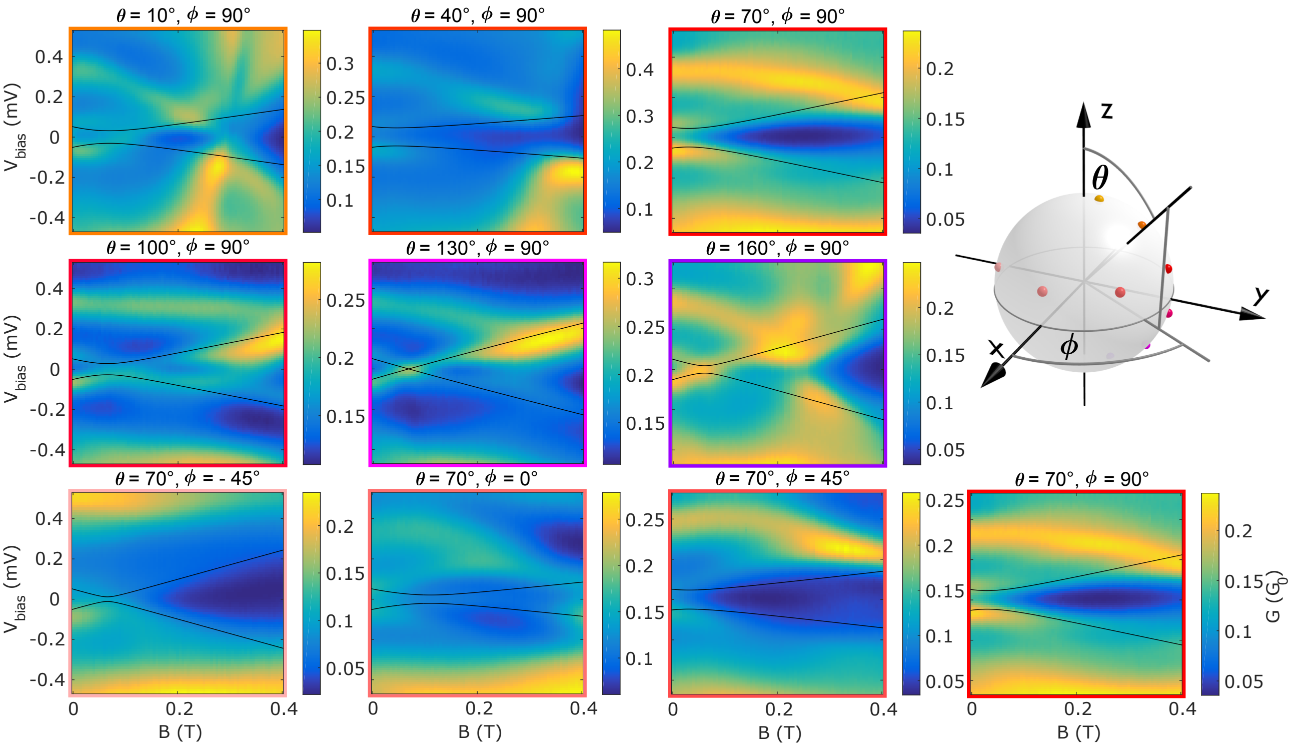


FIG. S2: Magnetic field dependence of the energy gap between the ground and first excited state of the (1,1) charging state, measured by inelastic cotunneling spectroscopy. Colors of the frames of the measurement panels refer to the magnetic field orientation, and corresponds to the balls indicated in the top right panel. Solid black lines show the gap as computed from a spin-orbit-coupled two-site Hubbard model (see Sec. III).

In the absence of magnetic field, the gap between the ground and first excited state is $\Delta E \approx J_0 \approx 0.055$ meV, reflected in the transport data in all subfigures of Fig. S2 by two conductance peaks positioned symmetrically around zero bias. The current is increased once the bias voltage reaches the energy necessary to excite the coupled double dot, thereby opening a new conduction channel via inelastic co-tunneling processes. This is reflected as the peak at $eV_{\mathrm{bias}} = \Delta E$ in the conductance. As the magnetic field increased, the excitation energy $\Delta E$ changes differently depending on the field direction (see Fig. S2). For certain directions (e.g. $\theta = 70°, \phi = 90°$), $\Delta E$ starts to increase almost immediately, while in others (e.g. $\theta = 100°, \phi = 90°$) the splitting first decreases and then starts to increase again after reaching a minimum. In the special direction, $\theta = 130°, \phi = 90°$, excitation lines cross at $B = 70$ mT, thereby forming a magnetic Weyl point. The degeneracy at the crossing point is further supported by the enhanced Kondo conductance, generated by strong coupling to the normal leads, and analyzed in detail in the main text.

In each panel of Fig. S2, the solid black lines show the gap between the ground state and the first excited state, as computed from a spin-orbit-coupled two-site Hubbard model. The model is described in Methods and in the next section of this Supplementary Information. The black lines describe the measured conductance ridge very well for most directions, taking into account that only three fitting parameters were used to fit all these characteristics (see details later). Though in certain cases, e.g., at $\theta = 70°$, $\phi = 45°$, the conductance ridges do not follow the solid black line but appear at higher energy.

In addition to the inelastic co-tunneling resonance reflecting the gap between the ground and first excited state within the (1,1) subspace, Fig. S2 also shows further resonances. At zero magnetic field, e.g., a resonance appears at

$V_{\rm bias} \approx 0.35$ mV, see, e.g., the top right subfigure ($\theta = 70°$, $\phi = 90°$) in Fig. S2. We attribute this line to the next accessible orbital level. The evolution of this excited state line also depends on the direction of the magnetic field. Further deviations between our simple model and the experiments can be caused by the fact that the g-tensors used in the $(1,1)$ state were determined from measurements carried out in the neighboring charge states $(0,1)$ and $(1,0)$ at different gate voltages, which may modify the $g$-tensors.[3,4]

## III. TWO-SITE HUBBARD MODEL OF THE DOUBLE QUANTUM DOT

To describe the presence of the magnetic Weyl points and the electronic energy spectrum of a double quantum dot, we use a spin-orbit-coupled two-site Hubbard-model, including magnetic field and spin-flip hopping. The Hamiltonian $H = H_0 + H_Z$ is specified in Methods.

Spin-orbit coupling is incorporated in the Hamiltonian via two different mechanisms. First, due to spin-orbit interaction (SOI), and the broken spatial symmetries arising from the fabrication and environment of the nanostructure, the electronic $g$-tensors in $H_Z$ for each dot are anisotropic and have uncontrolled principal values and directions. Note that even though we use the word 'spin' the single-electron basis states of this Hamiltonian are not spin states in the usual sense: instead, they are zero-field Kramers pairs, possessing an entangled spin and orbital character. Often this two-dimensional quantum degree of freedom is called *pseudospin*, or *spin-orbit qubit*.[5] Second, in the presence of SOI, interdot hopping is not expected to conserve spin, let alone pseudospin, and that is accounted for by the spin-flip tunneling terms in $H_0$. From now on we restrict our description to the double occupation of the double dot system, leaving 6 relevant states.

### A. Mapping the Hubbard model to two interacting spins

In the main text, one part of the discussion describes interacting localized spins, the other part describes a double quantum dot in which electrons can hop from one site to the other. It is well known that in the limit of strong on-site Coulomb repulsion, these two systems are related: the two-site Hubbard model can be mapped to two interacting spins using second-order perturbation theory. In the absence of SOI, this mapping results in an isotropic, Heisenberg-type antiferromagnetic interaction between the localized spins. In the presence of SOI, this interaction is more complicated: it incorporates anisotropic as well Dyaloshinskii-Moriya-type interaction terms. Here, we outline the derivation and the results of that mapping.

In the two-electron subspace, the Hamiltonian of the double dot is:

$$H_{6\times 6} = \begin{pmatrix} 2\varepsilon_L + U_L & -it_x + t_y & -t_0 + it_z & t_0 + it_z & it_x + t_y & 0 \\ it_x + t_y & \varepsilon_L + \varepsilon_R & 0 & 0 & 0 & it_x + t_y \\ -t_0 - it_z & 0 & \varepsilon_L + \varepsilon_R & 0 & 0 & -t_0 - it_z \\ t_0 - it_z & 0 & 0 & \varepsilon_L + \varepsilon_R & 0 & t_0 - it_z \\ -it_x + ty & 0 & 0 & 0 & \varepsilon_L + \varepsilon_R & -it_x + t_y \\ 0 & -it_x + t_y & -t_0 + it_z & t_0 + it_z & it_x + t_y & 2\varepsilon_R + U_R \end{pmatrix} . \quad \text{(S1)}$$

Here we ordered the basis states as $|\uparrow\downarrow, 0\rangle$, $|\uparrow,\uparrow\rangle$, $|\uparrow,\downarrow\rangle$, $|\downarrow,\uparrow\rangle$, $|\downarrow,\downarrow\rangle$, and $|0,\uparrow\downarrow\rangle$, the arrows representing the single-electron pseudospin basis states. This Hamiltonian can be easily diagonalized numerically.

Our double dot is in the regime of strong Coulomb repulsion, where the Coulomb energies $U_L$ and $U_R$ are much larger than the hopping amplitudes $t_0$, and $t_{x,y,z}$ that provide coupling within the (1,1)-(2,0) and (1,1)-(0,2) state pairs. We focus on this regime. We apply a second-order Schrieffer-Wolff transformation to eliminate the high-energy (2,0) and (0,2) states, and to obtain a $4 \times 4$ effective Hamiltonian restricted to the (1,1) subspace:

$$H_{4\times 4} = \frac{(t_0^2 + t_x^2 + t_y^2 + t_z^2)(U_L + U_R)}{(U_L + \varepsilon_L - \varepsilon_R)(U_R + \varepsilon_R - \varepsilon_L)} + \boldsymbol{S}_L \hat{\boldsymbol{J}} \boldsymbol{S}_R \, , \quad \text{(S2)}$$

where we have introduced the spin operators on the left/right, $\boldsymbol{S}_{L/R}$, and the following $3 \times 3$ exchange coupling matrix

$$\hat{\boldsymbol{J}} = \frac{U_L + U_R}{(U_L + \varepsilon_L - \varepsilon_R)(U_R + \varepsilon_R - \varepsilon_L)} \begin{pmatrix} t_0^2 + t_x^2 - t_y^2 - t_z^2 & 2(t_x t_y + t_0 t_z) & 2(t_x t_z - t_0 t_y) \\ 2(t_x t_y - t_0 t_z) & t_0^2 - t_x^2 + t_y^2 - t_z^2 & 2(t_y t_z + t_0 t_x) \\ 2(t_x t_z + t_0 t_y) & 2(t_y t_z - t_0 t_x) & t_0^2 - t_x^2 - t_y^2 + t_z^2 \end{pmatrix} . \quad \text{(S3)}$$

A few important remarks regarding this result are in order. (i) The first term in $H_{4\times 4}$ is just a constant energy shift. The second term in $H_{4\times 4}$ describes the exchange interaction between the two electrons residing in the two

dots. (ii) The exchange matrix $\hat{\boldsymbol{J}}$ in Eq. (S3) looks quite generic: it is neither symmetric nor antisymmetric. (iii) Nevertheless, $\hat{\boldsymbol{J}}$ is not fully generic. A fully generic exchange matrix is parametrized by 9 independent real numbers (the 9 matrix elements), and consequently, its spectrum consists of 4 non-degenerate energy levels unless some special symmetry induces degeneracies. However, $\hat{\boldsymbol{J}}$ in Eq. (S3) is characterized by 4 independent real numbers (a global scaling factor depending on $U_{L/R}$, $\varepsilon_{L/R}$ and $t_0$, and a three-dimensional vector $\boldsymbol{t}/t_0$), where $\boldsymbol{t} = (t_x, t_y, t_z)$, and has the special property that the ground state is non-degenerate and the first excited state is threefold degenerate. (iv) We emphasize that in the presence of spin-flip hopping (i.e. $\boldsymbol{t} \neq 0$), the unique ground state of $H_{4\times4}$ is *not* the usual 'pseudospin singlet' $\frac{1}{\sqrt{2}}(|\uparrow,\downarrow\rangle - |\downarrow,\uparrow\rangle)$, since in general the ground state includes all four states of the pseudospin product basis. However, it makes sense to call the ground state 'singlet' and the zero-field excited states 'triplets', not as a reference to their pseudospin state, but as a reference to their degrees of degeneracy.

### B. Determination of the Hubbard-model parameters from experimental data

Due to the strong tunnel coupling to the leads, charge states $(0,1)$ and $(1,0)$ in the double dot display the Kondo effect at zero magnetic field. This is revealed by the zero-bias conductance ridge in Fig. 2c of the main text, in the gate-voltage range $V_{\mathrm{gL}} \in [0.5, 0.515]$ V. This Kondo resonance shows a Zeeman splitting in a finite magnetic field, which in turn gives us a tool to determine the $g$-tensors of each dot individually.

Measured Zeeman-split Kondo resonances are presented in the panels of Fig. S3, which show the dependence of the conductance $G$ on magnetic field length $B$ and bias voltage $V_{\mathrm{bias}}$. Data were taken at the hexagon centers of the $(0,1)$ and $(1,0)$ charge states of the charge stability diagram (see Fig. 2b of main text), scanning different magnetic-field orientations, $\theta \in \{0°, 10°, \ldots, 180°\}$ and $\phi \in \{0°, 45°, 90°\}$. The panels in Fig. S3 show a selection of the measured conductance data in the (0,1) charge state. Colors of the panel frames correspond to the colored balls indicating the magnetic-field orientation in the bottom right panel of Fig. S3.

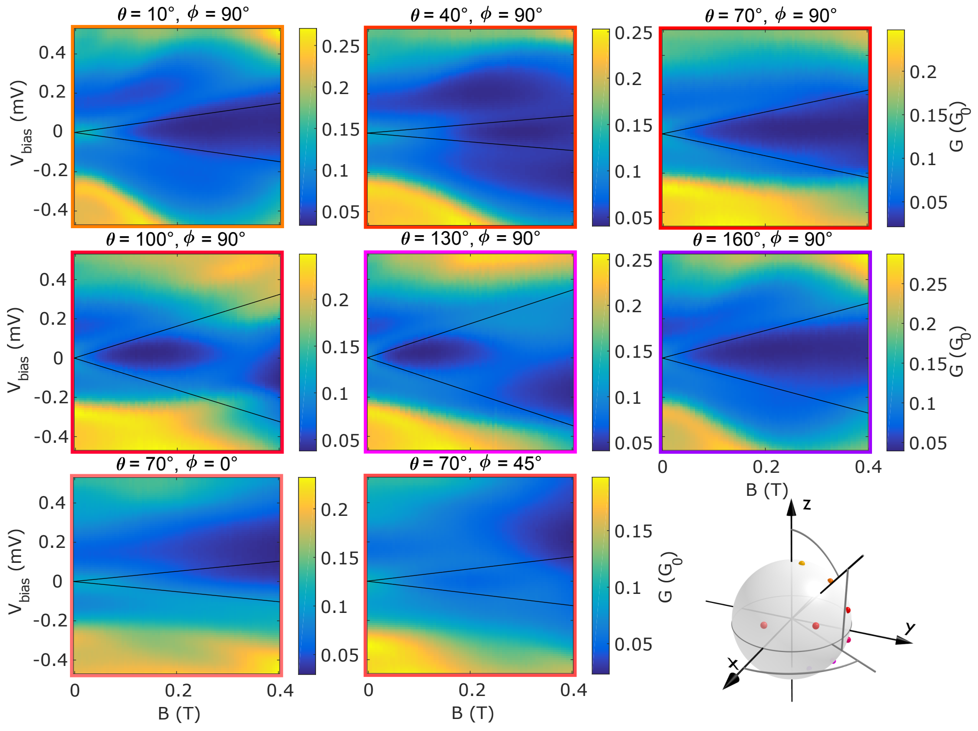


FIG. S3: Determining the $g$-factor of the right dot from the Zeeman splitting of the Kondo resonance in the (0,1) sector. Magnetic field directions are the same as in Fig. S2. Conductance is measured in units of $G_0 = 2e^2/h$. Colors of the frames refer to the magnetic field orientation, and correspond to the balls indicated in the bottom right panel.

At low magnetic fields, the distance between the Zeeman-split Kondo ridges in Fig. S3 seems to be proportional to the magnetic field, but for higher fields this linear dependence breaks down, for example when the Kondo resonance gets close to another excited state of the double dot, as seen in the middle panel of Fig. S3 with $\theta = 130°$ and $\phi = 90°$.

We determined the $g$-tensors using the low-field conductance data, where the Zeeman splitting of the two Kondo ridge is approximately linear in $B$. Here we identified the slopes of maxima and minima of $dG(V_{\mathrm{bias}}, B)/dV_{\mathrm{bias}}$ (i.e. the inflection point of the differential conductance).[6] These slopes are plotted in Fig. S4a and b separately for the two dots, and for the measured angles $\phi$. Then, we determine $\hat{\boldsymbol{g}}_{L/R}$ by fitting these values by the Zeeman splitting of the simple Zeeman Hamiltonian $H_{\mathrm{Z},L/R} = \mu_B \boldsymbol{B}\hat{\boldsymbol{g}}_{L/R}\boldsymbol{S}_{L/R}$, assuming $\hat{\boldsymbol{g}}_{L/R}$ is a real symmetric matrix. This procedure yields the two $g$-tensors specified in Methods.

The fitting procedure provides a very good agreement with experimental data as seen in Fig. S3 and S4a,b. In Fig. S3 the solid black line shows the Zeeman splitting of $H_{\mathrm{Z},R}$, and can be compared to the magnetic field dependence of the measured conductance resonances. While Fig. S4a & b present the overall comparison of the angle dependence of the experimental and fitted values of $|\hat{\boldsymbol{g}}\boldsymbol{B}|$/B for $\mathrm{QD_L}$ and $\mathrm{QD_R}$ respectively.

The two $g$-tensors are visualized in two different ways in Fig. S4c and d. Fig. S4c shows the dimensionless Zeeman splittings $|\hat{\boldsymbol{g}}_{L/R}\hat{\boldsymbol{B}}|$ where $\hat{\boldsymbol{B}} = \boldsymbol{B}/B$ is the unit vector along the magnetic field, for $\mathrm{QD_{L/R}}$. More precisely, the yellow/blue surface is the image of the unit sphere via the map $\hat{\boldsymbol{B}} \mapsto |\hat{\boldsymbol{g}}_{L/R}\hat{\boldsymbol{B}}|$. Fig. S4d shows the dimensionless effective magnetic fields $\hat{\boldsymbol{g}}_{L/R}\hat{\boldsymbol{B}}$. Note that the directions of the principal axes of the $g$-tensors are not related to the geometry of the sample.

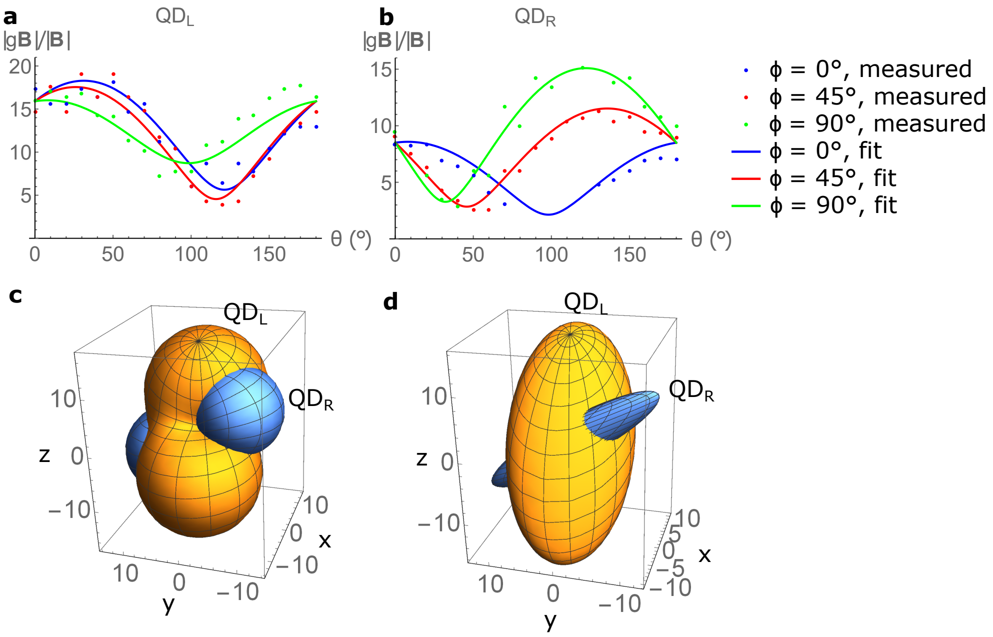


FIG. S4: Anisotropic $g$-tensors in the double quantum dot. **a**, **b**, Dots: Zeeman splittings extracted from the measured conductance data in the left (**a**) and right (**b**) dots. Solid lines: fitted Zeeman splittings using the Hamiltonian $H_{\mathrm{Z},L/R}$ (see text). **c**, Yellow/blue: Dimensionless Zeeman splitting in the left/right dot. **d**, Yellow/blue: Dimensionless effective magnetic field in the left/right dot. See text for definitions.

We have determined the on-site Coulomb interaction from the charge stability diagrams, giving $U_R \approx 1$ meV and $U_R \approx 0.6$ meV. In the experiments we have positioned our voltages to the center of the (1,1) region, corresponding to $\varepsilon_R = -U_R/2$ and $\varepsilon_L = -U_L/2$. Having fixed these four parameters, as well as all $g$-tensor elements using the procedure described above, only the four hopping amplitudes remain as fitting parameters. We have fixed these by two conditions: (1) our model has to reproduce the zero field splitting, $\Delta E_0 = 8(t_0^2 + \boldsymbol{t}^2)/(U_L + U_R)$, and (2) the two lowest energy eigenstates should cross for a magnetic field in the $\theta = 130°$, $\phi = 90°$ direction. The first condition fixes $t = \sqrt{t_0^2 + \boldsymbol{t}^2}$ to 0.105 meV, while the second condition gives two more restrictions on the hopping parameters, leaving one free parameter. Generated fits for all measured magnetic field directions with several different choices of the free parameter showed that the free parameter has a negligible effect on the liability of the fits. The hopping parameter values we used are listed in Methods. Having fixed all model parameters this way allows us to simulate the spectrum for any $\boldsymbol{B}$ field, and determine the splitting between the ground state and the first excited state. These energy differences are displayed as solid gray lines on panels d, e and f of Fig. 2 in the main text, and as solid black lines in Figs. S2 and S3.

### C. Symmetry of the $g$-tensor

In our spin-orbit coupled two-site Hubbard model, we assume that the $g$-tensors are symmetric matrices, see Methods and Sec. III B of this Supplementary Information. This is a valid starting point, even though in general a $g$-tensor does not have to be symmetric: using polar decomposition, any real invertible matrix can be written as the product of an orthogonal matrix $\mathcal{O}$ and a symmetric matrix: $\hat{\boldsymbol{g}} = \mathcal{O} \cdot \hat{\boldsymbol{g}}_{sym}$. The $\mathcal{O}$ transformation corresponds to a unitary transformation of the pseudospin basis. This transformation changes the tunnel amplitudes $(t_{0;x;y;z})$ in $H_0$ of the Hubbard model, but does not change the parametric form of the tunnel Hamiltonian, which is dictated by the time-reversal symmetry constraint. Therefore, our model is fully generic, despite the apparent restriction that the $g$-tensors are symmetric.

## IV. NUMERICAL CALCULATION OF THE TOPOLOGICAL CHARGE OF MAGNETIC WEYL POINTS

To illustrate the concept of the topological charges, let us consider a single spin-1/2 in a Zeeman field, described by the $2 \times 2$ Hamiltonian $H = \boldsymbol{B} \cdot \boldsymbol{S}$. Straightforward analytical calculations yield then a ground-state Berry curvature $\mathcal{B} = \boldsymbol{B}/(2B^2)$.[7] Therefore the ground-state Chern number for any sphere $\mathcal{S}_0$ centered around the origin is simply $C(\mathcal{S}_0) = 1$. The Berry curvature being divergence-free in any region where the ground state is non-degenerate, $C(\mathcal{S}) = 1$ holds for any closed surface enclosing the origin.

This result can be generalized if we allow for a non-trivial $g$-tensor $\hat{\boldsymbol{g}}$, $H = \mu_B \boldsymbol{B}\hat{\boldsymbol{g}}\boldsymbol{S}$. To have a well-defined Chern number for $\mathcal{S}_0$, the determinant of $\hat{\boldsymbol{g}}$ has to be nonzero: otherwise, $\hat{\boldsymbol{g}}$ has a vanishing principal value, which implies that the ground state is degenerate for magnetic fields along the corresponding principal axis. This line of singularities (degeneracies) prevents the evaluation of the Chern number at any closed surface around $\boldsymbol{B} = 0$. If $\det \hat{\boldsymbol{g}} \neq 0$, then we obtain $C(\mathcal{S}) = \operatorname{sign} \det \hat{\boldsymbol{g}}$. A way to show this is to consider simple limiting cases such as $\hat{\boldsymbol{g}} = \operatorname{diag}(1, 1, -1)$, e.g. analytically, and use the argument that the Chern number cannot jump as long as the $g$-tensor is continuously deformed such that its determinant does not reach zero.

Figure 2h of main text visualizes the topological charge of a degeneracy point ('magnetic Weyl point') by showing the normalized Berry curvature vector field. This plot is based on our spin-orbit coupled two-site Hubbard model, which is described in Methods and in section III of this Supplementary Information, using the parameters extracted from experimental data. The Berry curvature vector field plays the role of a magnetic field, and is created by the *degeneracy points* that play the role of 'magnetic charges' or 'magnetic monopoles'. Lines or surfaces of degeneracies can possess magnetic charge densities. The Chern number of a closed surface is analogous to the magnetic flux piercing that surface. Therefore, e.g., if the Berry curvature vector field shows an outward oriented hedgehog or skyrmion pattern around a degeneracy point, then it signals that its flux piercing a surrounding surface will be nonzero, which in turn indicates a finite Chern number for that surface. In this context, the magnetic charge carried by a degeneracy point can also be called a 'topological charge', because its value is quantized.

To illustrate the Berry curvature vector field in Fig. 2h of main text and Fig. S6 of the Supp. Mat., we calculate it approximately, numerically, on a cubic grid of magnetic field points, and plot the normalized Berry curvature $\mathcal{B}/|\mathcal{B}|$ in a few such grid points in the vicinities of the two magnetic Weyl points (red balls in Fig. 2h of main text). The procedure for the approximate numerical evaluation of the Cartesian components of the Berry curvature, e.g., $\mathcal{B}_z$, is as follows. The cubic grid is defined as the set of points $\{\boldsymbol{B}_{\boldsymbol{n}} \equiv \boldsymbol{n}\,\Delta \,|\, \boldsymbol{n} = (n_x, n_y, n_z) \in \mathbb{Z}^3\}$, with $\Delta$ the grid size in the magnetic field space. To estimate the Berry curvature component $\mathcal{B}_z$ at the grid point $\boldsymbol{n}\Delta$, consider the closed oriented square-shaped path in the magnetic field space that is defined by the loop of grid points

$$\begin{aligned}
\boldsymbol{B}_1 &= (n_x - 1, n_y - 1, n_z)\,\Delta, \\
\boldsymbol{B}_2 &= (n_x + 1, n_y - 1, n_z)\,\Delta, \\
\boldsymbol{B}_3 &= (n_x + 1, n_y + 1, n_z)\,\Delta, \\
\boldsymbol{B}_4 &= (n_x - 1, n_y + 1, n_z)\,\Delta.
\end{aligned}$$

We refer to the oriented square-shaped surface enclosed by this loop as $b$. For a fine grid, $\Delta \to 0$, the Berry curvature can be regarded as constant on $b$, and therefore it is a good approximation to approximate the Berry flux piercing the square $b$ (that is, the surface integral of the Berry curvature) as

$$\int_b d\boldsymbol{s} \cdot \mathcal{B} \approx 4\Delta^2 \mathcal{B}_z(\boldsymbol{n}) \,. \tag{S4}$$

On the other hand, the Berry flux is also well approximated by the discrete Berry phase associated to the four ground

states at the four corners of the square[7]:

$$\int_b d\boldsymbol{s}\cdot\boldsymbol{\mathcal{B}} \approx -\arg\mathrm{Tr}\left(P_1P_2P_3P_4\right) \tag{S5}$$

where $P_j$ $(j = 1,2,3,4)$ is the ground-state projector in corner $j$ of the square, that is, $P_j = |\psi_0(\boldsymbol{B}_j)\rangle\langle\psi_0(\boldsymbol{B}_j)|$. Combining Eqs. (S4) and (S5) as

$$\mathcal{B}_z(\boldsymbol{n}) \approx -\frac{1}{4\Delta^2}\arg\mathrm{Tr}\left(P_1P_2P_3P_4\right), \tag{S6}$$

we then use the numerically obtained ground states $\psi_0(\boldsymbol{B}_j)$ to approximate the Berry curvature components.

## V. STATISTICS AND STRUCTURE OF WEYL POINTS

### A. Statistics of Weyl points for random configurations

The topological considerations in the main text impose restrictions on the possible number of Weyl points, but cannot tell their exact number. Indeed, the 2 and 6 Weyl point situations are both topologically stable and robust, and it is a natural question, which one of them is more generic?

To determine the typical number of Weyl points, we made a statistical analysis by generating random Hubbard Hamiltonians with uniformly distributed parameters,

$$g_{\alpha,i}\in[1,5],\qquad U_\alpha\in[0.1,5],\qquad \{\alpha_L,\gamma_L\}\in[-\pi,\pi],\ \text{ and }\ \cos(\beta_L)\ \in\ [-1,1]. \tag{S7}$$

Here $\alpha_L$, $\beta_L$, and $\gamma_L$ denote Euler angles describing the rotated $g$-tensor of the left dot using the $ZYZ$ convention. Since only the relative orientation of $\hat{\boldsymbol{g}}_L$ and $\hat{\boldsymbol{g}}_R$ matters, we have set the Euler angles for $\mathrm{QD_R}$ to zero, $\alpha_R = \beta_R = \gamma_R = 0$. The hopping parameters $t_0, t_x, t_y, t_z$ were randomly chosen from the [-0.2,0.2] interval, but they were thrown away in case $t = \sqrt{t_0^2 + \boldsymbol{t}^2}$ was larger than 0.2, or smaller than 0.01.

For each parameter set, we identified the magnetic Weyl points of the $6\times 6$ Hamiltonian matrices corresponding to the two-electron subspace (see Methods). The statistics of the number of Weyl points for 2000 random configurations are shown in Table. I. For the choice of random parameters described above, the fraction of 6 Weyl point arrangements was roughly $\sim 0.5\%$, while in $\sim 99.5\%$ of the cases we found a single pair of Weyl points. We have not found more than six Weyl points among the 2000 random configurations, which would correspond to having degeneracies on a ring or sphere, confirming that such configurations can occur only for special parameter sets. We have repeated this analysis for the $4\times4$ exchange-coupled spin Hamiltonians $H_{4\times4}+H_Z$, which can be derived from the two-site Hubbard model, see Eq. S2. We considered the same 2000 random parameter sets as for the $6\times 6$ Hamiltonian matrices, and found identical results for the numbers of magnetic Weyl points.

| # of Weyl points | count |
|---|---|
| 2 | 1989 |
| 6 | 11 |
| 10+ | 0 |

TABLE I: Statistics of the number of Weyl points for 2000 random Hamiltonian configurations.

### B. Transition between configurations with different number of Weyl points

As it was discussed, both the 2 and 6 Weyl points configurations are topologically robust. In this subsection an example is given how the 6 Weyl points are transformed to 2 by tuning one of the spin flip hopping terms.

Figure S5 shows such a transition in detail. Two-site Hubbard model of Sec. III was used for the demonstration. In particular, we fixed $U_L = U_R = 1$ meV, $\varepsilon_L = \varepsilon_R = -U_L/2$, and assumed the following g-tensors,

$$\hat{\boldsymbol{g}}_L = \begin{pmatrix}1&0&0\\0&4&0\\0&0&7\end{pmatrix},\qquad \hat{\boldsymbol{g}}_R = \begin{pmatrix}6&0&0\\0&1&0\\0&0&3\end{pmatrix}, \tag{S8}$$

and the spin-flip hopping term was continuously enhanced from zero value ($\alpha = 0$) keeping the strength of the total hopping term fixed:

$$t_0 = 0.12\ \cos\alpha\ \text{meV},\ \ t_x = 0.12\ \sin\alpha\ \text{meV},\ \ \text{and}\ \ t_y = t_z = 0\ \text{meV}. \tag{S9}$$

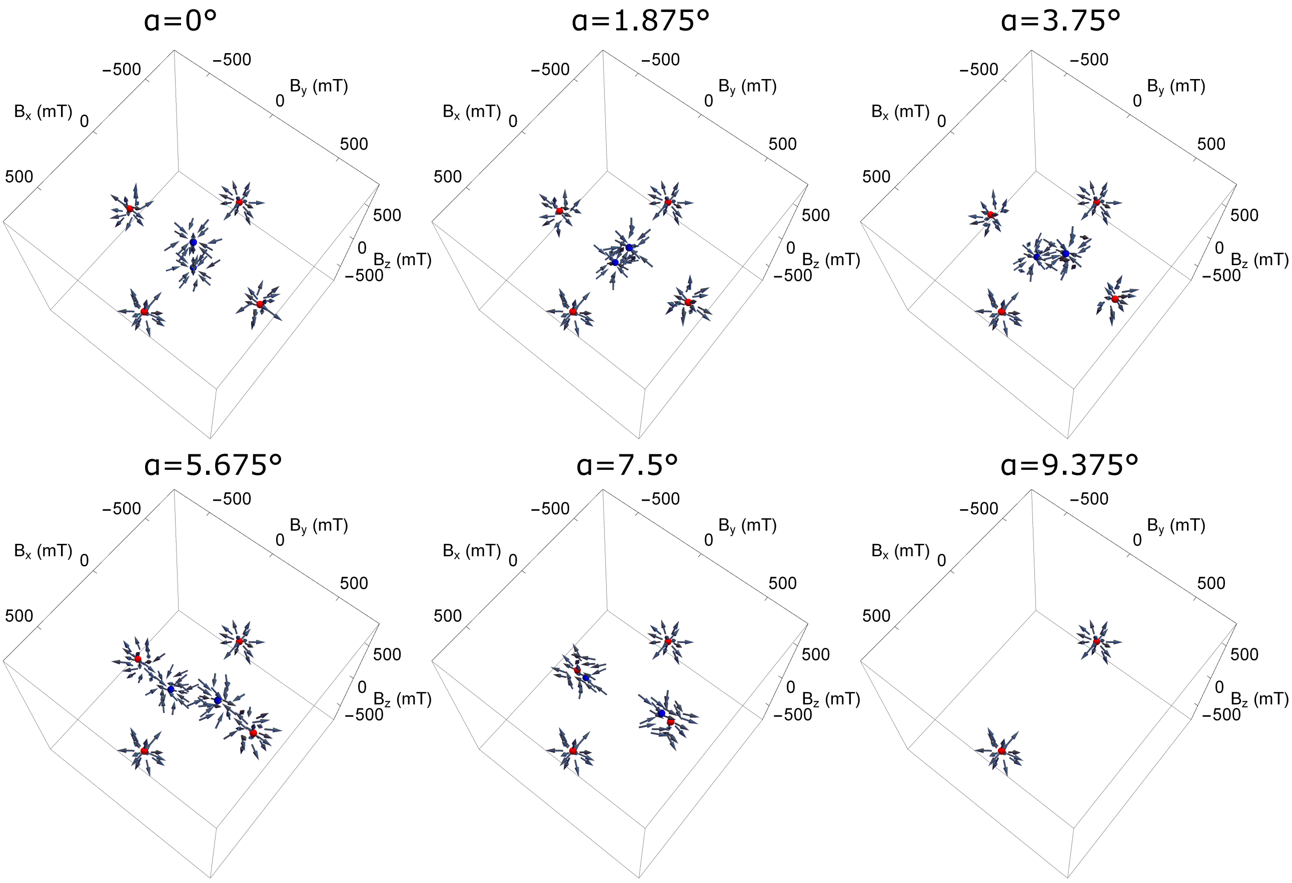


FIG. S5: $6 \rightarrow 2$ Weyl points transition via merging of Weyl points with opposite charge. Without spin flip hopping ($\alpha = 0$) 6 Weyl points are positioned along the coordinate axes, 4 with positive topological charge (red) and 2 with negative one (blue). The Berry curvature vector field is shown by arrows in the vicinity of the Weyl points. Turning on $t_x$, i.e. $\alpha > 0$ two pairs of Weyl points with opposite charge approach and annihilate each other.

For $\alpha = 0$ (see upper left panel of Fig. S5) six Weyl points positioned along the coordinate axes exist. The Berry curvature vector field was calculated as it is described in the previous subsection of the Supp. Mat. and shown by arrows in the vicinity of the Weyl points. The outward oriented hedgehog pattern indicate four positively charged Weyl points along the $x$ and $y$ axis (marked by red spots) and two negatively charged ones along the $z$ axis (marked by blue spots). As $\alpha$ is increased the blue Weyl points and the red Weyl points positioned along $y$ axis gradually shift in the $y - z$ plane and approach each other. For $\alpha = 7.63°$ the positively and negatively charged pairs of Weyl points annihilate and only two red Weyl points remain along the $x$ axis (see right bottom panel of Fig. S5).

Investigating various situations we have found that this annihilation process is the generic transition from 6 to 2 Weyl points. There are special cases e.g. when two pairs of Weyl points of opposite charge form a ring of degeneracies with 0 total topological charge. However such cases require special parameter set of the model and are not robust against perturbation.

---

[1] M. H. Madsen *et al.*, Journal of Crystal Growth **364**, 16 (2013).
[2] H. Shtrikman *et al.*, Nano Letters **9**, 1506 (2009), pMID: 19253998.

[3] S. Csonka *et al.*, Nano Lett. **8**, 3932 (2008).
[4] M. D. Schroer, K. D. Petersson, M. Jung, and J. R. Petta, Phys. Rev. Lett. **107**, 176811 (2011).
[5] S. Nadj-Perge, S. M. Frolov, E. P. A. M. Bakkers, and L. P. Kouwenhoven, Nature **468**, 1084 (2010).
[6] J. Paaske, A. Rosch, and P. Wölfle, Phys. Rev. B **69**, 155330 (2004).
[7] J. K. Asbóth, L. Oroszlány, and A. Pályi, *A Short Course on Topological Insulators* (Springer, ADDRESS, 2016).
